# Supplementary material for: Enhancing the ODMR Signal of Organic Molecular Qubits
Source: arXiv:2409.19249 ancillary file (2024-11-21)
Supplement: Supplementary file 1 [file Supplementary_Information.pdf]

Supplementary Information for

# Enhancing the ODMR Signal of Organic Molecular Qubits

Yong Rui Poh,[1,*] and Joel Yuen-Zhou[1,*]

[1]Department of Chemistry and Biochemistry, University of California San Diego, La Jolla, California 92093, USA
*Corresponding authors. Email addresses: ypoh@ucsd.edu (Y.R.P.); joelyuen@ucsd.edu (J.Y.-Z.)

## Contents

**S1 Rate equations for the microkinetic model** **2**

**S2 Estimate of the maximum optical pump rate** **2**

**S3 Results from ab initio calculations** **3**

S3.1 Benzyl-*p*-benzyl diradical . . . 3

S3.2 $PT_2TM$-*p*-$PT_2TM$ diradical . . . 3

S3.3 $Cl_4M$-*p*-$Cl_4M$ diradical . . . 8

S3.4 $PT_2TM$-H monoradical . . . 10

# S1 Rate equations for the microkinetic model

The rate equations are

$$\frac{d}{dt}\mathbf{N} = \mathbf{K}\mathbf{N}, \tag{S1}$$

where

$$\mathbf{N} \equiv \begin{pmatrix} n_{\mathrm{GS}} & n_{\mathrm{GT0}} & n_{\mathrm{GT1}} & n_{\mathrm{CT}} & n_{\mathrm{ES}} & n_{\mathrm{ES*}} & n_{\mathrm{ET0}} & n_{\mathrm{ET1}} & n_{\mathrm{ET*0}} & n_{\mathrm{ET*1}} \end{pmatrix}^{\mathrm{T}} \tag{S2}$$

is a column vector containing the eigenstate populations, and

$$\mathbf{K} \equiv \mathrm{diag}\begin{pmatrix} -2k_{\mathrm{abs}} - 3k_{\mathrm{decoh}} \\ -2k_{\mathrm{abs}} - k_{\mathrm{decoh}} - 2\kappa_{\mathrm{decoh}} \\ -4k_{\mathrm{abs}} - k_{\mathrm{decoh}} - \kappa_{\mathrm{decoh}} \\ -k_{\text{CT-GS}} - 4k_{\text{CT-ET}} - k_{\text{CT-GT}}/2 \\ -2k_{\text{ES-CT}} - 2k_{\text{ES-GT}} - 6k_{\mathrm{decoh}} \\ -2k_{\mathrm{VR}} - k_{\mathrm{abs}} \\ -k_{\text{ET-GT}} - 2k_{\mathrm{decoh}} - 4\kappa_{\mathrm{decoh}} \\ -2k_{\text{ET-CT}} - k_{\text{ET-GS}} - 2k_{\text{ET-GT}} - 2k_{\mathrm{decoh}} - 2\kappa_{\mathrm{decoh}} \\ -2k_{\mathrm{VR}} - k_{\mathrm{abs}} \\ -4k_{\mathrm{VR}} - 2k_{\mathrm{abs}} \end{pmatrix}$$
$$+ \begin{pmatrix} 0 & k_{\mathrm{decoh}} & k_{\mathrm{decoh}} & k_{\text{CT-GS}} & 0 & k_{\mathrm{abs}} & 0 & k_{\text{ET-GS}} & 0 & 0 \\ k_{\mathrm{decoh}} & 0 & \kappa_{\mathrm{decoh}} & k_{\text{CT-GT}}/2 & 0 & 0 & k_{\text{ET-GT}} & 0 & k_{\mathrm{abs}} & 0 \\ 2k_{\mathrm{decoh}} & 2\kappa_{\mathrm{decoh}} & 0 & 0 & 2k_{\text{ES-GT}} & 0 & 0 & 2k_{\text{ET-GT}} & 0 & 2k_{\mathrm{abs}} \\ 0 & 0 & 0 & 0 & 2k_{\text{ES-CT}} & 0 & 0 & 2k_{\text{ET-CT}} & 0 & 0 \\ 0 & 0 & 0 & 0 & 0 & 2k_{\mathrm{VR}} & 2k_{\mathrm{decoh}} & 2k_{\mathrm{decoh}} & 0 & 0 \\ 2k_{\mathrm{abs}} & 0 & 0 & 0 & 0 & 0 & 0 & 0 & 0 & 0 \\ 0 & 0 & 0 & 0 & 2k_{\mathrm{decoh}} & 0 & 0 & 2\kappa_{\mathrm{decoh}} & 2k_{\mathrm{VR}} & 0 \\ 0 & 0 & 0 & 4k_{\text{CT-ET}} & 4k_{\mathrm{decoh}} & 0 & 4\kappa_{\mathrm{decoh}} & 0 & 0 & 4k_{\mathrm{VR}} \\ 0 & 2k_{\mathrm{abs}} & 0 & 0 & 0 & 0 & 0 & 0 & 0 & 0 \\ 0 & 0 & 4k_{\mathrm{abs}} & 0 & 0 & 0 & 0 & 0 & 0 & 0 \end{pmatrix} \tag{S3}$$

is a matrix containing the rate constants. Note the factor of 1/2 accompanying $k_{\text{CT-GT}}$, which is needed because this ISC occurs only from the $^1\mathrm{CT}_A$ state. Also, we have defined the diag operator by

$$\mathrm{diag}\ (a_1, a_2, \cdots, a_j, \cdots)^{\mathrm{T}} \equiv \begin{pmatrix} a_1 & & & & \\ & a_2 & & & \\ & & \ddots & & \\ & & & a_j & \\ & & & & \ddots \end{pmatrix}. \tag{S4}$$

# S2 Estimate of the maximum optical pump rate

We estimate the pump rate $k_{\mathrm{abs}}$ using the Einstein $B$ coefficient to be

$$k_{\mathrm{abs}} = \frac{e^2 \rho(\nu)}{4\epsilon_0 m_{\mathrm{e}} h\nu} f_{\mathrm{osc}}, \tag{S5}$$

where $\nu$ and $f_{\mathrm{osc}}$ are the frequency and oscillator strength of the transition in question, and $\rho(\nu)$ is the spectral energy density of the radiation field at frequency $\nu$. The remaining symbols are constants with $e$ for the elementary charge, $\epsilon_0$ for the vacuum permittivity, $m_{\mathrm{e}}$ for the electron mass, and $h$ for the Planck constant. To obtain $\rho(\nu)$, we considered a teaching lab set-up [1], which focused a 532 nm Thorlabs DJ532-40 laser with a power $P$ of 40 mW onto a diameter $2r$ of $10\,\mu$m. We further assumed the lineshape to be flat around the peak frequency and zero elsewhere; the linewidth $\delta\nu$ was estimated from the user manual to be around 30 MHz. Then, a crude estimate of $\rho(\nu)$ would be

$$\rho(\nu) \approx \frac{P}{c\pi r^2 \delta\nu} = 5.67 \times 10^{-8}\,\mathrm{J\,m^{-3}\,Hz^{-1}}, \tag{S6}$$

where $c$ is the speed of light. Taking $\nu$ to be the frequency corresponding to 532 nm wavelength light, we obtain the following upper bound to the pump rate:

$$k_{\text{abs}} \lesssim \left(1.21 \times 10^{14}\,\text{s}^{-1}\right) f_{\text{osc}}. \tag{S7}$$

$f_{\text{osc}}$ for the lowest-lying excitation of trityl-based radicals is typically around 0.01 [2], hence

$$k_{\text{abs}} \lesssim 10^{12}\,\text{s}^{-1}. \tag{S8}$$

# S3 Results from ab initio calculations

## S3.1 Benzyl-*p*-benzyl diradical

The triplet SCF calculation converged to an energy of −14692.84714 eV and an $\langle \mathbf{S}^2 \rangle$ value of 2.066128. The level of theory was UB3LYP-D3BJ/def2-SVP.

### Relaxed geometry

```
C        0.00000      -0.00000       0.74467
C        0.85600       0.85600       1.46798
C        0.86047       0.86047       2.85451
C        0.00000      -0.00000       3.60202
C       -0.86047      -0.86047       2.85451
C       -0.85600      -0.85600       1.46798
C        0.00000      -0.00000       5.00984
C        0.00000       0.00000      -0.74467
C       -0.85600       0.85600      -1.46798
C       -0.86047       0.86047      -2.85451
C        0.00000       0.00000      -3.60202
C        0.86047      -0.86047      -2.85451
C        0.85600      -0.85600      -1.46798
C        0.00000       0.00000      -5.00984
H        1.53268       1.53268       3.39476
H       -1.53268      -1.53268       3.39476
H        1.52419       1.52419       0.91856
H       -1.52419      -1.52419       0.91856
H        0.66239       0.66239       5.57165
H       -0.66239      -0.66239       5.57165
H       -1.52419       1.52419      -0.91856
H       -1.53268       1.53268      -3.39476
H        1.53268      -1.53268      -3.39476
H        1.52419      -1.52419      -0.91856
H        0.66239      -0.66239      -5.57165
H       -0.66239       0.66239      -5.57165
```

## S3.2 $\mathbf{PT_2TM}$-*p*-$\mathbf{PT_2TM}$ diradical

At the UB3LYP-D3BJ/def2-SVP level, the triplet SCF calculation converged to an energy of −289833.13523 eV and an $\langle \mathbf{S}^2 \rangle$ value of 2.042099. At the UB3LYP/def2-SVPD level, the triplet SCF calculation converged

to an energy of −289830.85584 eV and an $\langle \mathbf{S}^2 \rangle$ value of 2.042475, while the BS SCF calculation converged to an energy of −289830.85637 eV and an $\langle \mathbf{S}^2 \rangle$ value of 1.043240.

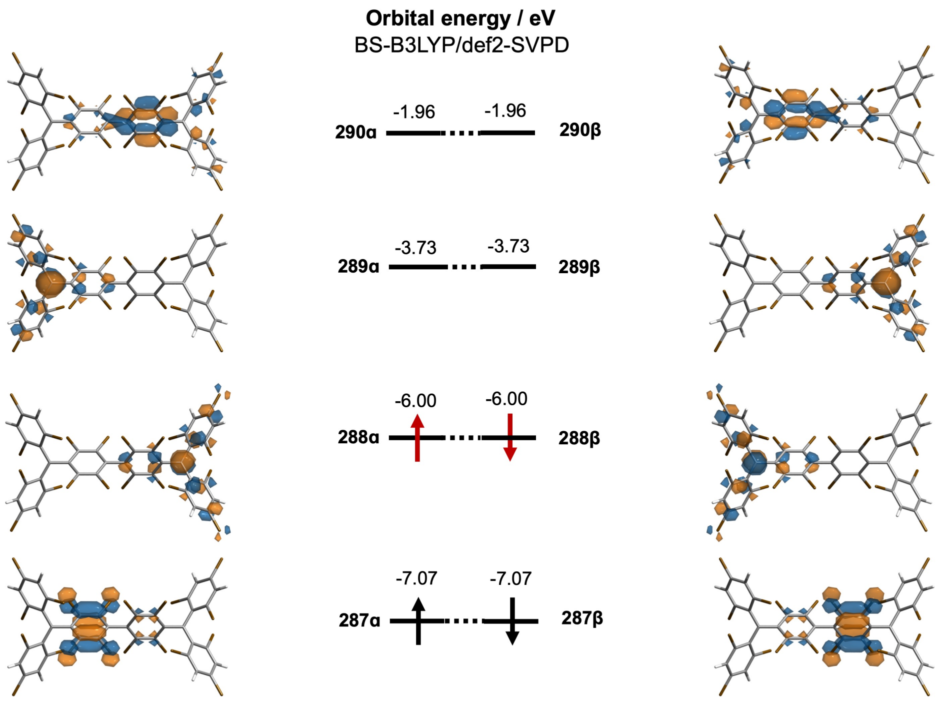


**FIG. S1**: Frontier MOs (isovalue = 0.040) of $PT_2TM$-$p$-$PT_2TM$ in the open-shell BS ground state, calculated at the BS-B3LYP/def2-SVPD level.

## Optimised geometry

| | | | |
|---|---|---|---|
| C | -0.00000574198939 | 0.00001886283277 | -0.74318861439021 |
| C | -0.82678095278225 | -0.88014609927434 | -1.45536400066426 |
| Cl | -1.86258482682735 | -1.95194106627830 | -0.56444113784991 |
| C | -0.83158350247726 | -0.88052339029383 | -2.85590319631644 |
| Cl | -1.95524855748238 | -1.91142816496441 | -3.68705975754690 |
| C | -0.00000581608866 | 0.00001070235900 | -3.58709128147569 |
| C | -0.00000299485762 | 0.00000270365669 | -5.06000657824186 |
| C | 0.83157078934871 | 0.88055023033315 | -2.85590840237393 |
| Cl | 1.95523778087506 | 1.91144805135712 | -3.68707097425392 |
| C | 0.82676835945782 | 0.88018086804408 | -1.45536905544954 |
| Cl | 1.86257456143681 | 1.95197859168642 | -0.56445230199539 |
| C | -0.00000217001731 | 0.00001886023804 | 0.74318883337673 |
| C | -0.82677472934388 | 0.88018224539217 | 1.45536943291133 |
| Cl | -1.86258005949903 | 1.95198119702163 | 0.56445301708662 |
| C | -0.83157635775357 | 0.88055200382982 | 2.85590876820934 |
| Cl | -1.95524159458849 | 1.91145152361032 | 3.68707165578374 |
| C | -0.00000037868010 | 0.00001166522908 | 3.58709138684470 |
| C | -0.00000217031194 | 0.00000400182907 | 5.06000668839507 |
| C | 0.83157573883127 | -0.88052373037234 | 2.85590315107515 |
| Cl | 1.95523992781849 | -1.91142956821651 | 3.68705956373061 |
| C | 0.82677228466328 | -0.88014698607087 | 1.45536398549090 |
| Cl | 1.86257439566614 | -1.95194342327608 | 0.56444084701128 |
| C | 0.17900551702102 | 1.26105603892104 | 5.78366664773472 |

```
C   1.18654999229765      2.19790973989786   5.43741456569588
Cl  2.34674782212454      1.83644445241497   4.18400725246410
C   1.35578328747814      3.40684333867228   6.10821255653891
C   0.50637407962282      3.71770775388578   7.17018267287389
Cl  0.70601325535163      5.22457207778832   8.01770385285598
C   -0.50173341875719      2.83484933278354    7.55989016889500
C   -0.65389520593741      1.63504372449640    6.86985291974398
Cl  -1.99962191524371      0.62889321298102    7.34263264520852
C   -0.17900731381876     -1.26105719724744    5.78365132901835
C   0.65389603742513     -1.63505770789699   6.86983115658126
Cl  1.99962002055447     -0.62890949357922   7.34262357276859
C   0.50173985908195     -2.83487427268144   7.55985059808921
C   -0.50636443216016     -3.71773102480600    7.17013096038665
Cl  -0.70599589518047     -5.22460914677200    8.01762938869358
C   -1.35577635243562     -3.40685394272176    6.10816672444608
C   -1.18654882214552     -2.19790949292590    5.43738678478131
Cl  -2.34674901230920     -1.83643049144512    4.18398555581708
C   -0.17900758247265      1.26105489983025     -5.78366697668087
C   0.65389622129251      1.63504114729646     -6.86985133538927
Cl  1.99962136494639      0.62888751881681     -7.34262894868841
C   0.50173892567358      2.83484762634097     -7.55988803632161
C   -0.50636691203772      3.71770851048111     -7.17018180219864
Cl  -0.70599985874512      5.22457422381186     -8.01770195128842
C   -1.35577896714643      3.40684562968217     -6.10821351254259
C   -1.18655038448497      2.19791090446352     -5.43741629119332
Cl  -2.34675149392943      1.83644779362864     -4.18401136732756
C   0.17900538028328     -1.26105804288897     -5.78365098915979
C   1.18655104625317     -2.19790638119409     -5.43738774456401
Cl  2.34675168860653     -1.83642266135838     -4.18398831465705
C   1.35578318435328     -3.40684960143919     -6.10816867440069
C   0.50637160709494     -3.71772954726441     -7.17013232856319
Cl  0.70600875240596     -5.22460635065789     -8.01763178908284
C   -0.50173704243424     -2.83487703443063     -7.55985028577585
C   -0.65389753780493     -1.63506141783068     -6.86983015992414
Cl  -1.99962641341773     -0.62891874914231     -7.34262045883576
H   2.15383251571159      4.08730443443524   5.81464959278671
H   -1.17756531411163      3.08516224915109    8.37639864788383
H   1.17757398010457     -3.08519688520980   8.37635426492385
H   -2.15382312551000     -4.08731387719391    5.81459441988635
H   1.17757314063382      3.08515940411222     -8.37639495110400
H   -2.15382680646866      4.08730873330317     -5.81465144967596
H   2.15383311378736     -4.08730637419219     -5.81459757501016
H   -1.17757097095111     -3.08520213298905     -8.37635336504712
```

**Triplet excited states from UB3LYP/TDDFT/TDA/def2-SVPD**

```
STATE  1:  E=   0.093149 au  2.535 eV    20443.8 cm**-1 <S**2> =   2.128548
   282b -> 288b  :     0.057155 (c=  0.23907088)
   283b -> 287b  :     0.083378 (c=  0.28875206)
   285b -> 288b  :     0.348725 (c= -0.59052963)
   286b -> 287b  :     0.457583 (c=  0.67644853)
STATE  2:  E=   0.093205 au  2.536 eV    20456.0 cm**-1 <S**2> =   2.128185
```

```
   282b -> 287b  :     0.063197 (c= -0.25138950)
   283b -> 288b  :     0.083895 (c= -0.28964616)
   285b -> 287b  :     0.397785 (c=  0.63070190)
   286b -> 288b  :     0.400775 (c= -0.63306814)
STATE  3:  E=   0.096181 au  2.617 eV    21109.3 cm**-1 <S**2> =   2.169460
   287a -> 290a  :     0.021460 (c= -0.14649167)
   288a -> 289a  :     0.028774 (c=  0.16962792)
   277b -> 288b  :     0.037751 (c=  0.19429633)
   281b -> 288b  :     0.335959 (c=  0.57961952)
   284b -> 287b  :     0.520854 (c= -0.72170183)
STATE  4:  E=   0.096859 au  2.636 eV    21258.1 cm**-1 <S**2> =   2.173917
   287a -> 289a  :     0.038217 (c=  0.19549194)
   288a -> 290a  :     0.035136 (c= -0.18744546)
   277b -> 287b  :     0.033009 (c= -0.18168410)
   281b -> 287b  :     0.373787 (c= -0.61138117)
   284b -> 288b  :     0.465990 (c=  0.68263493)
STATE  5:  E=   0.096945 au  2.638 eV    21276.9 cm**-1 <S**2> =   2.150603
   287a -> 292a  :     0.028892 (c=  0.16997656)
   288a -> 291a  :     0.024328 (c= -0.15597515)
   282b -> 288b  :     0.351610 (c= -0.59296688)
   283b -> 287b  :     0.375825 (c= -0.61304560)
   285b -> 288b  :     0.035408 (c= -0.18816884)
   286b -> 287b  :     0.133565 (c=  0.36546515)
STATE  6:  E=   0.097079 au  2.642 eV    21306.4 cm**-1 <S**2> =   2.150283
   287a -> 291a  :     0.024191 (c= -0.15553573)
   288a -> 292a  :     0.030420 (c=  0.17441401)
   282b -> 287b  :     0.378789 (c=  0.61545844)
   283b -> 288b  :     0.344036 (c=  0.58654606)
   285b -> 287b  :     0.054106 (c=  0.23260648)
   286b -> 288b  :     0.119298 (c= -0.34539516)
STATE  7:  E=   0.104197 au  2.835 eV    22868.6 cm**-1 <S**2> =   2.125107
   287a -> 291a  :     0.012208 (c=  0.11049073)
   288a -> 293a  :     0.012435 (c= -0.11151433)
   279b -> 287b  :     0.471603 (c= -0.68673332)
   280b -> 288b  :     0.437931 (c= -0.66176332)
   282b -> 287b  :     0.012287 (c=  0.11084545)
STATE  8:  E=   0.104205 au  2.836 eV    22870.3 cm**-1 <S**2> =   2.124973
   287a -> 293a  :     0.012500 (c= -0.11180518)
   288a -> 291a  :     0.012225 (c=  0.11056768)
   279b -> 288b  :     0.434934 (c=  0.65949515)
   280b -> 287b  :     0.474013 (c=  0.68848638)
   282b -> 288b  :     0.011371 (c= -0.10663722)
   283b -> 287b  :     0.011275 (c= -0.10618423)
```

ABSORPTION SPECTRUM VIA TRANSITION ELECTRIC DIPOLE MOMENTS

| State | Energy (cm-1) | Wavelength (nm) | fosc | T2 (au**2) | TX (au) | TY (au) | TZ (au) |
|---|---|---|---|---|---|---|---|
| 1 | 20443.8 | 489.1 | 0.003282776 | 0.05286 | 0.22991 | -0.00163 | -0.00000 |
| 2 | 20456.0 | 488.9 | 0.019409525 | 0.31237 | -0.00069 | -0.55890 | 0.00005 |
| 3 | 21109.3 | 473.7 | 0.060043138 | 0.93641 | -0.00003 | 0.00005 | -0.96768 |
| 4 | 21258.1 | 470.4 | 0.000000020 | 0.00000 | 0.00016 | -0.00052 | -0.00009 |

| | | | | | | | | |
|---|---|---|---|---|---|---|---|---|
| 5 | 21276.9 | 470.0 | 0.000801065 | 0.01239 | 0.11133 | 0.00083 | -0.00019 |
| 6 | 21306.4 | 469.3 | 0.061450615 | 0.94949 | -0.00010 | 0.97442 | 0.00010 |
| 7 | 22868.6 | 437.3 | 0.005164043 | 0.07434 | -0.00696 | -0.27257 | 0.00004 |
| 8 | 22870.3 | 437.2 | 0.011462876 | 0.16501 | 0.40618 | -0.00466 | 0.00004 |

### Singlet excited states from BS-B3LYP/TDDFT/TDA/def2-SVPD

```
STATE  1:  E=   0.072498 au  1.973 eV    15911.4 cm**-1 <S**2> =   0.182750
   287a -> 288a  :     0.440292 (c=  0.66354522)
   287b -> 288b  :     0.555762 (c= -0.74549461)
STATE  2:  E=   0.072512 au  1.973 eV    15914.6 cm**-1 <S**2> =   0.181942
   287a -> 288a  :     0.555944 (c= -0.74561668)
   287b -> 288b  :     0.440475 (c= -0.66368284)
STATE  3:  E=   0.093217 au  2.537 eV    20458.7 cm**-1 <S**2> =   1.128499
   284a -> 288a  :     0.074182 (c=  0.27236462)
   285a -> 288a  :     0.059299 (c=  0.24351293)
   286a -> 288a  :     0.349276 (c=  0.59099606)
   284b -> 288b  :     0.071064 (c= -0.26657893)
   285b -> 288b  :     0.056877 (c=  0.23848921)
   286b -> 288b  :     0.334941 (c= -0.57874068)
STATE  4:  E=   0.093249 au  2.537 eV    20465.8 cm**-1 <S**2> =   1.129617
   284a -> 288a  :     0.073716 (c=  0.27150602)
   285a -> 288a  :     0.057721 (c=  0.24025234)
   286a -> 288a  :     0.331261 (c=  0.57555284)
   284b -> 288b  :     0.076815 (c=  0.27715504)
   285b -> 288b  :     0.060221 (c= -0.24540067)
   286b -> 288b  :     0.345538 (c=  0.58782483)
STATE  5:  E=   0.096325 au  2.621 eV    21140.9 cm**-1 <S**2> =   1.166153
   278a -> 288a  :     0.012457 (c=  0.11160882)
   281a -> 288a  :     0.078066 (c=  0.27940275)
   283a -> 288a  :     0.352531 (c= -0.59374329)
   287a -> 289a  :     0.020073 (c= -0.14168042)
   278b -> 288b  :     0.012411 (c=  0.11140512)
   281b -> 288b  :     0.078090 (c=  0.27944607)
   283b -> 288b  :     0.351778 (c= -0.59310870)
   287b -> 289b  :     0.020113 (c= -0.14182153)
STATE  6:  E=   0.096800 au  2.634 eV    21245.1 cm**-1 <S**2> =   1.175258
   281a -> 288a  :     0.076101 (c=  0.27586331)
   283a -> 288a  :     0.343482 (c= -0.58607367)
   287a -> 289a  :     0.031310 (c=  0.17694758)
   281b -> 288b  :     0.076389 (c= -0.27638594)
   283b -> 288b  :     0.343945 (c=  0.58646847)
   287b -> 289b  :     0.031262 (c= -0.17681019)
STATE  7:  E=   0.097041 au  2.641 eV    21298.0 cm**-1 <S**2> =   1.150917
   284a -> 288a  :     0.359091 (c= -0.59924219)
   286a -> 288a  :     0.087502 (c=  0.29580779)
   287a -> 291a  :     0.024935 (c=  0.15790760)
   284b -> 288b  :     0.353061 (c= -0.59418932)
   286b -> 288b  :     0.086024 (c=  0.29329775)
   287b -> 291b  :     0.025363 (c= -0.15925665)
STATE  8:  E=   0.097082 au  2.642 eV    21307.0 cm**-1 <S**2> =   1.151071
   284a -> 288a  :     0.354277 (c=  0.59521151)
```

```
   286a -> 288a  :     0.084660 (c= -0.29096448)
   287a -> 291a  :     0.026324 (c=  0.16224807)
   284b -> 288b  :     0.360305 (c= -0.60025406)
   286b -> 288b  :     0.086093 (c=  0.29341546)
   287b -> 291b  :     0.025886 (c=  0.16089062)
STATE  9:  E=   0.104217 au  2.836 eV    22872.9 cm**-1 <S**2> =   1.125907
   280a -> 288a  :     0.511958 (c=  0.71551211)
   284a -> 288a  :     0.012066 (c=  0.10984483)
   280b -> 288b  :     0.397747 (c= -0.63067226)
   287b -> 291b  :     0.011606 (c= -0.10773213)
STATE 10:  E=   0.104226 au  2.836 eV    22875.0 cm**-1 <S**2> =   1.125839
   280a -> 288a  :     0.397434 (c= -0.63042366)
   287a -> 291a  :     0.011375 (c= -0.10665240)
   280b -> 288b  :     0.511638 (c= -0.71528872)
   284b -> 288b  :     0.012492 (c= -0.11176961)
-----------------------------------------------------------------------------
         ABSORPTION SPECTRUM VIA TRANSITION ELECTRIC DIPOLE MOMENTS
-----------------------------------------------------------------------------
State   Energy    Wavelength  fosc         T2        TX        TY        TZ
        (cm-1)      (nm)                 (au**2)    (au)      (au)  (au)
-----------------------------------------------------------------------------
   1   15911.4    628.5   0.000009813   0.00020  -0.00000   0.00000   0.01425
   2   15914.6    628.4   0.002904789   0.06009  -0.00000  -0.00000   0.24513
   3   20458.7    488.8   0.019443057   0.31287   0.00239  -0.55934   0.00004
   4   20465.8    488.6   0.003239369   0.05211   0.22820   0.00583   0.00000
   5   21140.9    473.0   0.059563393   0.92754   0.00002   0.00005   0.96309
   6   21245.1    470.7   0.000000015   0.00000  -0.00002   0.00028  -0.00040
   7   21298.0    469.5   0.000872328   0.01348   0.11605   0.00413  -0.00012
   8   21307.0    469.3   0.061700546   0.95333   0.00049  -0.97638  -0.00000
   9   22872.9    437.2   0.005190136   0.07470  -0.02564   0.27211  -0.00002
  10   22875.0    437.2   0.011509315   0.16564   0.40663   0.01714   0.00004
```

## S3.3 $Cl_4$M-*p*-$Cl_4$M diradical

The triplet SCF calculation converged to an energy of −114701.41640 eV and an $\langle \mathbf{S}^2 \rangle$ value of 2.075353. The level of theory was UB3LYP-D3BJ/def2-SVP.

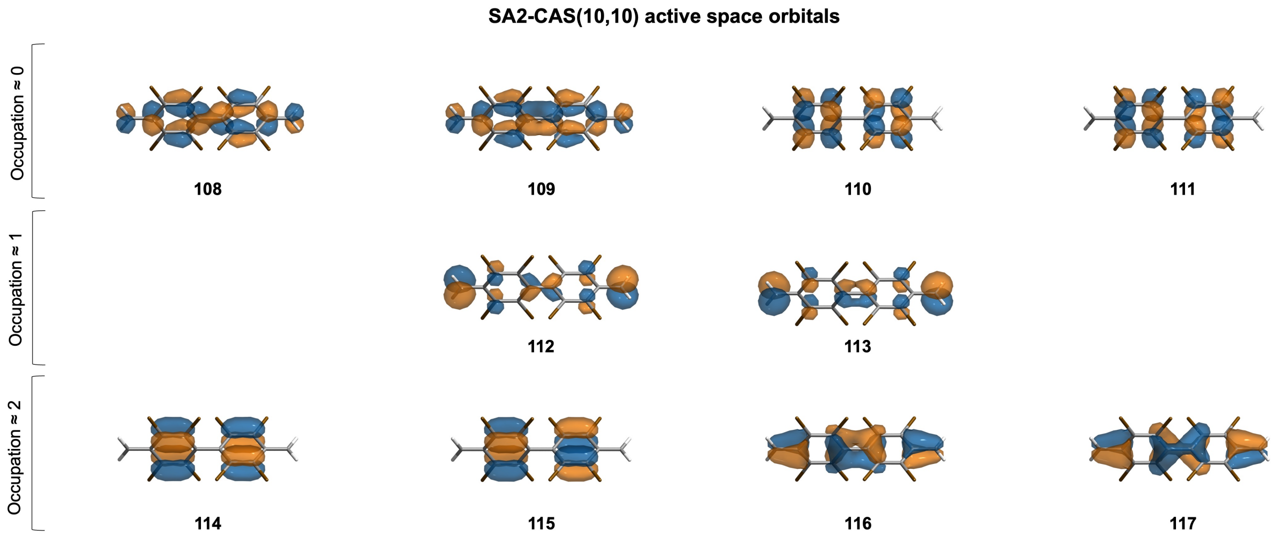


**FIG. S2**: Active space MOs (isovalue = 0.040) of $Cl_4$M-*p*-$Cl_4$M from a CASSCF(10,10)/def2-SVPD calculation state-averaged over the triplet and singlet ground states (i.e. SA2).

**Table S1**: Excited-state properties of $Cl_4$M-*p*-$Cl_4$M, calculated at the SA2-CASSCF(10,10)/CASCI/SC-NEVPT2/def2-SVPD level. The triplet and singlet $LE_{B_2}$ states are dominated by the following transitions: 114 → 113, 115 → 112, 113 → 111, 112 → 110. The triplet and singlet $LE_{B_3}$ states are dominated by the following transitions: 114 → 112, 115 → 113, 112 → 111, 113 → 110.

| Triplets | | Singlets | |
|---|---|---|---|
| **Energy / eV** | **Assignment** | **Energy / eV** | **Assignment** |
| 0.006 | $^3GS_{B_1}$ | 0.000 | $^1GS_A$ |
| | | 1.617 | $^1CT_A$ |
| | | 1.622 | $^1CT_{B_1}$ |
| 2.604 | $^3LE_{B_2}$ | 2.612 | $^1LE_{B_2}$ |
| 2.604 | $^3LE_{B_3}$ | 2.612 | $^1LE_{B_3}$ |

## Optimised geometry

```
C   0.00000041285253    0.00000029555640   0.74297677529495
C   0.85732573641907    0.85732631288620   1.46036723377016
C   0.86449831678849    0.86449897249083   2.85373875414654
Cl  1.93779307205256    1.93779488416541   3.69549743130807
C   -0.00000014382067   -0.00000005359037   3.61203276227255
C   -0.00000040175185   -0.00000028309773   5.01220248078794
C   -0.86449833501065   -0.86449887424287   2.85373817543095
Cl  -1.93779341609317   -1.93779493750990   3.69549621346067
C   -0.85732522342353   -0.85732588248186   1.46036665514901
Cl  1.90872191143777    1.90872327279931   0.56204835859350
Cl  -1.90872102502467   -1.90872254490025   0.56204699493039
H   0.66403776579042    0.66403836065583   5.56214484145260
H   -0.66403867943697   -0.66403921249331   5.56214434734771
C   0.00000059154361    0.00000047708230   -0.74297680842324
C   -0.85732498072283    0.85732650236958   -1.46036693763725
Cl  -1.90872068612633    1.90872347952667   -0.56204752525952
```

```
C   -0.86449821272356     0.86449900828024    -2.85373843687065
Cl  -1.93779350464977     1.93779467711227    -3.69549669018358
C   -0.00000016226542    -0.00000015609920    -3.61203278430882
C   -0.00000070594291    -0.00000065316442    -5.01220250752925
C    0.86449845299473    -0.86449884127681    -2.85373851575171
Cl   1.93779309206189    -1.93779501603972    -3.69549697710167
C    0.85732597981825    -0.85732568976200    -1.46036699911219
Cl   1.90872202824070    -1.90872234501100    -0.56204762706680
H    0.66403725680076    -0.66403966557926    -5.56214462005595
H   -0.66403913980843     0.66403791232367    -5.56214459464441
```

## S3.4 $PT_2TM$-H monoradical

The doublet SCF calculation converged to an energy of −144932.58265 eV and an $\langle \mathbf{S}^2 \rangle$ value of 0.770696. The level of theory was UB3LYP-D3BJ/def2-SVP.

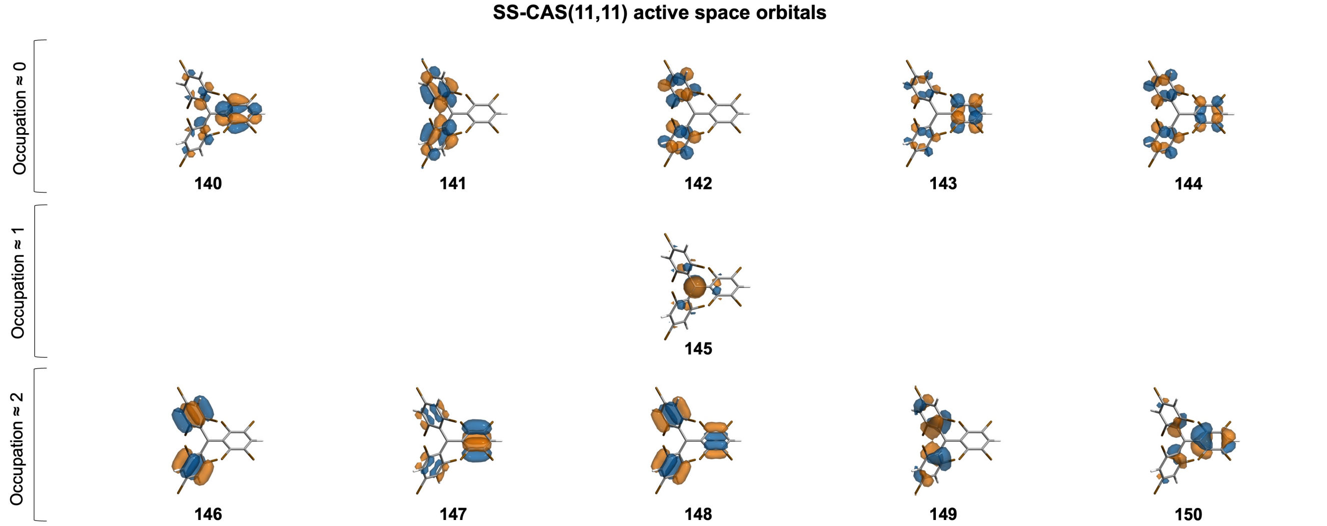


**FIG. S3**: Active space MOs (isovalue = 0.040) of $PT_2TM$-H from a CASSCF(11,11)/def2-SVPD calculation state-specific to the ground doublet.

**Table S2**: Excited-state properties of $PT_2TM$-H, calculated at the SS-CASSCF(11,11)/CASCI/SC-NEVPT2/def2-SVPD level.

| Energy / eV | Main contribution | Assignment |
|---|---|---|
| 0.000 | – | $^2$GS$_B$ |
| 2.780 | 147 → 145 | $^2$LE$_A$ |
| 2.988 | 146 → 145 | $^2$LE$_B$ |
| 3.078 | 149 → 145 | $^2$LE$_A$ |
| 3.296 | 150 → 145 | $^2$LE$_B$ |

### Optimised geometry

```
C   -0.00000100878170     0.00000169583685     4.12761634902078
C   -0.85851151864839    -0.84825523996764     3.42970609427926
```

| | | | |
|---|---|---|---|
| Cl | -1.92674366505162 | -1.87460275292160 | 4.33649252936941 |
| C | -0.86593552020095 | -0.85043019279702 | 2.02751198441216 |
| Cl | -2.02880823448355 | -1.83842286789924 | 1.19812103091070 |
| C | 0.00000078223341 | -0.00000051292764 | 1.29728867140791 |
| C | 0.00000068858206 | -0.00000072793933 | -0.17626186450116 |
| C | 0.86593621128483 | 0.85043028720999 | 2.02751182881201 |
| Cl | 2.02880918443113 | 1.83842267932249 | 1.19812093592387 |
| C | 0.85851038281088 | 0.84825754834784 | 3.42970593743530 |
| Cl | 1.92674044220314 | 1.87460731220680 | 4.33649225374461 |
| H | -0.00000190376054 | 0.00000268662313 | 5.21685381496298 |
| C | -0.12598996386433 | 1.26578433548672 | -0.90410738379568 |
| C | 0.72838903626060 | 1.60545985538092 | -1.98454582181853 |
| Cl | 2.04360888115442 | 0.55206219939831 | -2.43980438625745 |
| C | 0.62212380120034 | 2.80591663776188 | -2.68244689972772 |
| C | -0.35989860412666 | 3.72341732904067 | -2.30653883135869 |
| Cl | -0.50466198860348 | 5.23000087113262 | -3.16590016424509 |
| C | -1.22733044492931 | 3.44765896661459 | -1.24944541387940 |
| C | -1.10390077055072 | 2.23733510764173 | -0.57129516226888 |
| Cl | -2.28661969547178 | 1.91766442755174 | 0.67187747918888 |
| C | 0.12599048854006 | -1.26578580916702 | -0.90410764623741 |
| C | 1.10390190812176 | -2.23733651837442 | -0.57129696102111 |
| Cl | 2.28662214563588 | -1.91766617759692 | 0.67187451667678 |
| C | 1.22733129011585 | -3.44765996512256 | -1.24944800338326 |
| C | 0.35989862743596 | -3.72341798012113 | -2.30654085170079 |
| Cl | 0.50466181794816 | -5.23000100911267 | -3.16590313167695 |
| C | -0.62212426204596 | -2.80591724030012 | -2.68244763865872 |
| C | -0.72838916842485 | -1.60546084978066 | -1.98454578265692 |
| Cl | -2.04360934075232 | -0.55206304737579 | -2.43980314450043 |
| H | 1.31251887555110 | 3.02906092760722 | -3.49460860037946 |
| H | -2.00486979890244 | 4.15580546212846 | -0.96671010777986 |
| H | 2.00487110610469 | -4.15580639100197 | -0.96671381080138 |
| H | -1.31251978101571 | -3.02906104688623 | -3.49460909226058 |

# References


[1] H. Zhang, C. Belvin, W. Li, J. Wang, J. Wainwright, R. Berg, and J. Bridger, American Journal of Physics **86**, 225 (2018).

[2] Y. R. Poh, D. Morozov, N. P. Kazmierczak, R. G. Hadt, G. Groenhof, and J. Yuen-Zhou, Journal of the American Chemical Society **146**, 15549 (2024).
